# Supplementary material for: Quark mass effects in two-loop Higgs amplitudes
Source: arXiv:2001.06295 source file (2020-04-23)
Supplement: Supplementary file 1 [file results_qqbH.tex]

\begin{align}
-&\frac{i}{m_b^3} M_{y_t,2}^{fin}=
	\frac{16 \left(1+x^4\right) H_{-4}(x)}{3 x \left(-1+x^2\right)}
	-\frac{26 (1+x)^2 \log\left(\frac{\mu ^2}{m_b^2}\right){}^2}{x}
	\nonumber \\
	&
	-\frac{2 \pi ^2 (1049+x (-708+x (-2764+x (684+1355 x))))}{81 x \left(-1+x^2\right)}
	-\frac{32 \left(1+x^2\right) H_2(x){}^2}{9 x}
	\nonumber \\
	&
	-\frac{4 (17+x (-23+13 x (13+5 x))) H_3(x)}{9 x (1+x)}
	+\frac{4}{9} \left(92+\frac{107}{x}+59 x+\frac{144}{1+x}\right) \zeta_{3}
	\nonumber \\
	&
	-\frac{4 \pi ^2 (5+x (8+5 x)) \log(1+x)}{9 x}
	+\frac{(5+x (-54+x (-192+x (-54+125 x)))) \log(x)^4}{54 x \left(-1+x^2\right)}
	\nonumber \\
	&
	+\frac{64 (-1+x) (1+x (5+x)) H_{2,1}(x)}{3 x (1+x)}
	-\frac{8 (5+x (8+5 x)) H_{-3}(x)}{9 x}
	\nonumber \\
	&
	+\frac{(8+8 x (-18+x (-24+(-18+x) x))) H_4(x)}{3 x \left(-1+x^2\right)}
	-\frac{8993 (1+x)^2}{54 x}
	\nonumber \\
	&
	+H_{-2}(x) \left(-\frac{128 (1+x) \left(1+x^2\right)}{9 (-1+x) x}-\frac{\pi ^2 \left(88-40 x^4\right)}{27 x-27 x^3}-\frac{64 \left(1+x^2\right) H_2(x)}{9 x}\right)
	\nonumber \\
	&
	+\left(-\frac{4 (-1+x) (625+x (1292+625 x))}{27 x (1+x)}+\frac{16 \pi ^2 (4+x (27+x (25+(27-2 x) x)))}{27 x \left(-1+x^2\right)}\right) H_2(x)
	\nonumber \\
	&
	+\pi ^4 \left(-\frac{32}{15}-\frac{49}{15 (-1+x)}-\frac{277}{405 x}+\frac{31 x}{15}+\frac{1}{1+x}\right)
	\nonumber \\
	&
	+\log(1-x) \left(-\frac{4 (41+x (110+41 x))}{9 x}+\frac{\pi ^2 (-52+4 x (-1+x (91+31 x)))}{9 x (1+x)}
	\right.
	\nonumber \\
	&
	\left.
	-\frac{16 \pi ^2 \left(-1+x^2\right) \log(x)}{3 x}+\left(\frac{248}{9}+\frac{2}{x}+\frac{50 x}{3}-\frac{16}{1+x}\right) \log(x)^2-\frac{16 \left(-1+x^2\right) \log(x)^3}{3 x}
	\right.
	\nonumber \\
	&
	\left.
	+\left(32-\frac{88}{3 x}+\frac{88 x}{3}-\frac{64}{1+x}\right) H_2(x)\right)
	+\log\left(1+x^2\right)^2 \left(\frac{32 (1+x)^2}{9 x}+\frac{16 \pi ^2 \left(-1+x^2\right)}{27 x}
	\right.
	\nonumber \\
	&
	\left.
	+\frac{16 \left(-1+x^2\right) H_2(x)}{9 x}\right)
	+\log\left(\frac{\mu ^2}{m_b^2}\right) \left(-\frac{350 (1+x)^2}{3 x}
	\right.
	\nonumber \\
	&
	\left.
	-\frac{8 \pi ^2 (31+x (24+x (-116+x (12+25 x))))}{27 x \left(-1+x^2\right)}-\frac{16 (1+x (10+x)) \log(1-x)}{3 x}
	\right.
	\nonumber \\
	&
	\left.
	+\frac{(62+2 x (24+x (-134+x (-24+7 x)))) \log(x)^2}{9 x-9 x^3}+\frac{8 (1+x)^2 \log\left(1+x^2\right)^2}{3 x}
	\right.
	\nonumber \\
	&
	\left.
	+\log(x) \left(\frac{8}{3} \left(18+\frac{16}{-1+x}+\frac{1}{x}+x\right)+\frac{32 (1+x) \left(1+x^2\right) \log(1+x)}{3 (-1+x) x}-\frac{32 x (1+x) \log\left(1+x^2\right)}{3 (-1+x)}\right)
	\right.
	\nonumber \\
	&
	\left.
	-\frac{32 (1+x) \left(1+x^2\right) H_{-2}(x)}{3 (-1+x) x}-\frac{8 (-1+x) (31+x (86+31 x)) H_2(x)}{9 x (1+x)}\right)
	\nonumber \\
	&
	+\log(x)^2 \left(\frac{2}{27} \pi ^2 \left(\frac{1}{x}+51 x-\frac{6 (9+x (10+9 x))}{-1+x^2}\right)
	\right.
	\nonumber \\
	&
	\left.
	+\frac{533+x (-659+x (-1864+3 x (296+(233-175 x) x)))}{27 (-1+x)^2 x (1+x)}-\frac{4 (5+x (8+5 x)) \log(1+x)}{9 x}
	\right.
	\nonumber \\
	&
	\left.
	+\frac{4 \left(-1+x^2\right) \log\left(1+x^2\right)^2}{9 x}-\frac{8 \left(-3+x^4\right) H_{-2}(x)}{9 x \left(-1+x^2\right)}+\frac{16 \left(4-7 x^2+4 x^4\right) H_2(x)}{9 x-9 x^3}\right)
	\nonumber \\
	&
	+\log(x)^3 \left(-\frac{2 (34+x (82+x (-139+x (2+65 x))))}{27 x \left(-1+x^2\right)}+\frac{16 \left(1+x^2\right) \log(1+x)}{9 x}
	\right.
	\nonumber \\
	&
	\left.
	-\frac{16}{9} x \log\left(1+x^2\right)\right)+\log(x) \left(\frac{4 (69+x (138+41 x))}{9 (-1+x)}
	\right.
	\nonumber \\
	&
	\left.
	-\frac{8 \pi ^2 (11+(-1+x) x (-29+x (-1+16 x)))}{27 x \left(-1+x^2\right)}+\frac{8 \left(1+x^4\right) \zeta_{3}}{9 x-9 x^3}
	\right.
	\nonumber \\
	&
	\left.
	+\frac{32 \left(1+x^4\right) H_{-3}(x)}{9 x-9 x^3}
	\right.
	\nonumber \\
	&
	\left.
	+\frac{8 (5+x (8+5 x)) H_{-2}(x)}{9 x}+\frac{4}{3} \left(52+\frac{17}{x}+11 x-\frac{24}{1+x}\right) H_2(x)
	\right.
	\nonumber \\
	&
	\left.
	+\log\left(1+x^2\right) \left(-\frac{64 \pi ^2 x}{27}-\frac{128 x (1+x)}{9 (-1+x)}-\frac{64}{9} x H_2(x)\right)
	\right.
	\nonumber \\
	&
	\left.
	+\log(1+x) \left(\frac{64 \pi ^2 \left(1+x^2\right)}{27 x}+\frac{128 (1+x) \left(1+x^2\right)}{9 (-1+x) x}+\frac{64 \left(1+x^2\right) H_2(x)}{9 x}\right)
	\right.
	\nonumber \\
	&
	\left.
	+\frac{32 \left(1+x^4\right) H_3(x)}{9 x \left(-1+x^2\right)}\right)
\end{align}
